# Supplementary material for: Wild Visual Navigation: Fast Traversability Learning via Pre-Trained Models and Online Self-Supervision
Source: arXiv:2404.07110 source file (2024-04-10)
Supplement: Supplementary file 1 [file appendix.tex]

\section{Ablations}
\label{appendix:ablations}
Full-page images with examples

\section{Platform description}
\label{appendix:supervision-signal}

\matias{DINO computation time on different platforms}

\section{Supervision signal}
\label{appendix:supervision-signal}

\subsection{Supervision Signal}
\matias{If we are not highlighting this, I would rather explain this in the supervision generation section, and show more real examples in the Appendix}
Plot different trajectories for different trav metrics
